# Supplementary material for: Foundations of Multisensory Artificial Intelligence
Source: arXiv:2404.18976 source file (2024-04-29)
Supplement: Supplementary file 1 [file alg_supp.tex]

\begin{figure*}[tbp]
    \centering
    \begin{minipage}{0.55\textwidth}
    \vspace{-0mm}
    \begin{algorithm}[H]
    \begin{algorithmic}
    \REQUIRE Multimodal dataset $\{\mathbf{X_1}, \mathbf{X_2}$\}.
    \vspace{.2em}\hrule\vspace{.5em}
    \STATE $\theta$, $\phi$ $\leftarrow$ Initialize network parameters.
    \WHILE{not converged}
    \STATE $\{\vx_1, \vx_2\}$ $\leftarrow$ Sampled batch from $\{\mathbf{X_1}, \mathbf{X_2}$\}
    \STATE $\theta$ $\leftarrow$ Update parameters by maximizing $\mathcal{L}_{\textsc{\names}}$
    \FOR{$i=1$ to $k$}
    \STATE $\{\vx_1', \vx_2'\}$ $\leftarrow$ Sampled batch from $\{\mathbf{X_1}, \mathbf{X_2}$\}
    \STATE $\phi$ $\leftarrow$ Update parameters by maximizing $\mathcal{L}_{\textsc{NCE}}$
    \ENDFOR
    \ENDWHILE
    \RETURN $\theta$, $\phi$
  \end{algorithmic}
  \caption{CL training with sampling}
  \label{alg:training}
\end{algorithm}
\end{minipage}
\end{figure*}
