# Supplementary material for: Foundations of Multisensory Artificial Intelligence
Source: arXiv:2404.18976 source file (2024-04-29)
Supplement: Supplementary file 2 [file additional.tex]

\begin{table*}[t]
\centering
\fontsize{9}{11}\selectfont
\setlength\tabcolsep{2pt}
\caption{Additional experiments on CIFAR10~\cite{Krizhevsky} and MNIST~\cite{deng2012mnist} datasets using our \names\ objectives on image classification.}
\centering
\begin{tabular}{l|c c c}
\hline \hline
Task & \textsc{CIFAR10} & \textsc{MNIST}\\
\hline
SimCLR~\cite{chen2020simple} & 87.0\% & 98.84\%\\
SupCon~\cite{khosla2020supervised} & 92.7\% & 99.38\%\\
\names-SUP & 91.3\% & 99.21\%\\
\hline \hline
\end{tabular}
\label{tab:additional}
\end{table*}
