# Supplementary material for: Foundations of Multisensory Artificial Intelligence
Source: arXiv:2404.18976 source file (2024-04-29)
Supplement: Supplementary file 4 [file cmi_lower_appendix.tex]

\begin{table*}[t]
\centering
\fontsize{9}{11}\selectfont
\setlength\tabcolsep{4pt}
% \vspace{-3mm}
\caption{We verify our conditional lower and upper bound estimators on a synthetic dataset with fixed dimension of representation $d_z$ and varying number of samples $n$.}
\centering

\begin{tabular}{l|cccc}
\hline \hline
Number of samples ($\times 10^3$), $d_z=20$ & 5 & 10 & 20 & 50 \\
\hline
CCMI (MI-Diff + Classifier) & 2.03 & 2.06 & 2.15 & 2.20\\
Conditional InfoNCE & 2.19 & 2.20 & 2.20 & 2.20 \\
Conditional InfoNCE-CLUB & 3.45 & 3.53 & 2.98 & 2.86 \\
True CMI & 2.32 & 2.32 & 2.32 & 2.32\\
\hline \hline
\end{tabular}

\vspace{-2mm}
\label{tab:cmi_lower_supp}
\end{table*}
