# Supplementary material for: Foundations of Multisensory Artificial Intelligence
Source: arXiv:2404.18976 source file (2024-04-29)
Supplement: Supplementary file 5 [file cmi_upper_appendix.tex]

\begin{table}[t]
\centering
\fontsize{9}{11}\selectfont
\setlength\tabcolsep{4pt}
\caption{We verify our conditional lower and upper bound estimators on a synthetic dataset with varying dimensions of representation $d_z$ and fixed number of samples $n$.}
\centering

\begin{tabular}{l|ccccc}
\hline \hline
Dimension $d_z$, $n=2\times10^4$ & 1 & 10 & 20 & 50 & 100\\
\hline
CCMI (MI-Diff + Classifier) & 2.30 & 2.18 & 2.15 & 1.98 & 1.67\\
Conditional InfoNCE & 2.18 & 2.20 & 2.20 & 2.26 & 2.30\\
Conditional InfoNCE-CLUB & 3.70 & 2.95 & 2.98 & 2.79 & 2.86 \\
True CMI & 2.32 & 2.32 & 2.32 & 2.32 & 2.32 \\
\hline \hline
\end{tabular}

\label{tab:cmi_upper_supp}
\end{table}
